# Supplementary material for: Efficient Decentralized Deep Learning by Dynamic Model Averaging
Source: arXiv:1807.03210 source file (2018-11-13)
Supplement: Supplementary file 1 [file appendixRefs.tex]

\newlabel{app:sec:exps}{{A}{}{}{appendix.A}{}}

\newlabel{app:ssec:black_box}{{A.5}{5}{}{appendix.A}{}}
\newlabel{app:ssec:scale_out}{{A.6}{6}{}{appendix.A}{}}

\newlabel{app:sec:theory}{{B}{}{}{appendix.B}{}}
